# Supplementary material for: Communicate to Play: Pragmatic Reasoning for Efficient Cross-Cultural Communication in Codenames
Source: arXiv:2408.04900 source file (2024-08-09)
Supplement: Supplementary file 1 [file data_analysis.tex]

\section{Data analysis across clue giver attributes}
\label{sec:additional-embedding-results}

We attempt to see if the obtained clusters align with existing classes of clue givers that are recorded in the data set. We consider the following labels: \textit{nativeness} - (whether one is an English native speaker or not), \textit{political leaning} (conservative, moderate conservatism, libertarian, moderate liberal, liberal), \textit{race} (Asian, Black, Native American, Hispanic/Latino, White), \textit{conscientious} (a score in range 1-4), and \textit{gender} (male or female). Unfortunately, as we illustrate in \Cref{fig:pca-gender-pol} for political leaning and gender, we haven't found classes that significantly align with any of the K-Mean clusters. While it is possible that we have not run these tests with classes that would display such an alignment, it is also possible that the clusters are formed by features that involve non-trivial interactions between the socio-cultural background information variables. 
It is also possible that this misalignment is driven by class imbalances within the dataset. For example, we found that approximately 70\% of the contributors were White, leaving little room for the other races. In this case, the contribution to the total variance of the dataset coming from the minorities may be insignificant, and thus lost in PCA projections.   
This is further confirmed by our linear probing experiments (see \Cref{tab:lp}); here, using the representations projected onto the first 5 PCA dimensions, we train logistic-regression (linear) classifiers and contrast them with the fraction of the data occupied by the majority class. We find that the accuracies at convergence follow closely simply that of the fixed majority vote.

\begin{table}[htbp]
    \centering
    \small
    \begin{tabular}{p{1cm}ccc|c} %
        \toprule
         & \textbf{GloVE\_t-h} & \textbf{GPT\_t-h} & \textbf{GPT\_r} & \textbf{Majority} \\
        \midrule
        \textbf{nativeness} & \textbf{0.766} & 0.759  & 0.762 & 0.765 \\
        \textbf{political} & 0.38 & \textbf{0.397} & 0.387 & 0.386 \\
        \textbf{race} & 0.676 & \textbf{0.692} & 0.667 & 0.685 \\
        \textbf{consc.} & 0.353 & 0.336 & \textbf{0.356} & 0.356 \\
        \textbf{gender} & 0.518 & \textbf{0.556} & 0.525 & 0.551 \\
        \bottomrule
    \end{tabular}
        \caption{Accuracy scores of a logistic regression (linear) classifier, averaged over 5 random seeds, together with the proportion of the data occupied by the majority of a considered class. The features were derived from GloVE \textit{target}-\textit{hint}, GPT \textit{target}-\textit{hint}, and GPT \textit{rationale}.}
        \label{tab:lp}
    \vspace{-1.5em} %
\end{table}

\begin{figure}
  \centering
  \begin{subfigure}[b]{0.45\linewidth}
    \includegraphics[width=\linewidth]{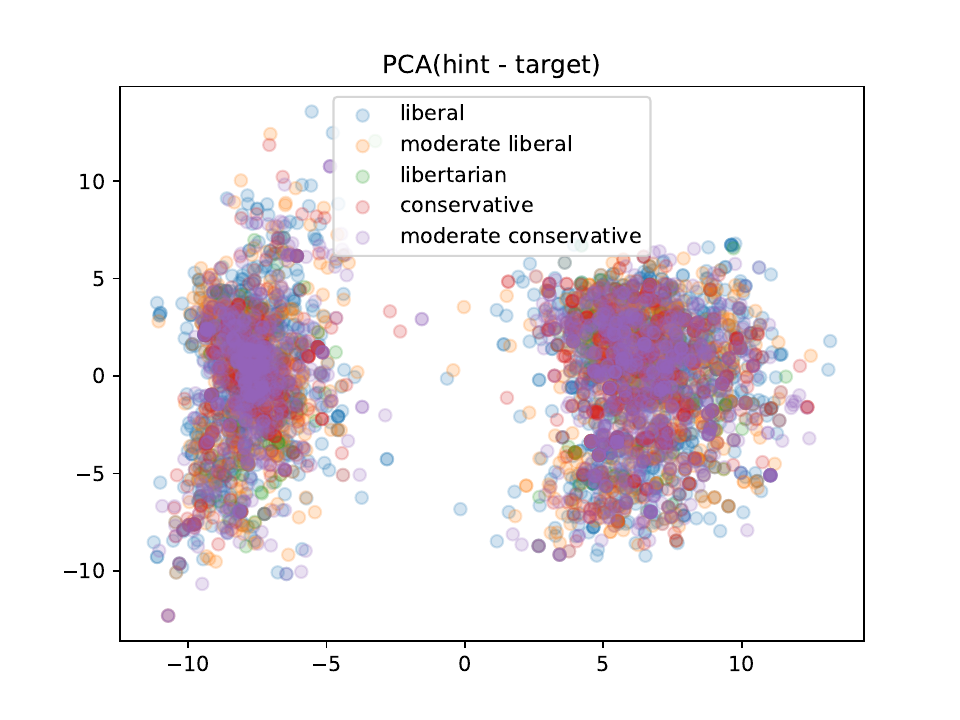}
    \caption{Political leaning}
    \label{fig:cos-glove}
  \end{subfigure}
  \begin{subfigure}[b]{0.45\linewidth}
    \includegraphics[width=\linewidth]{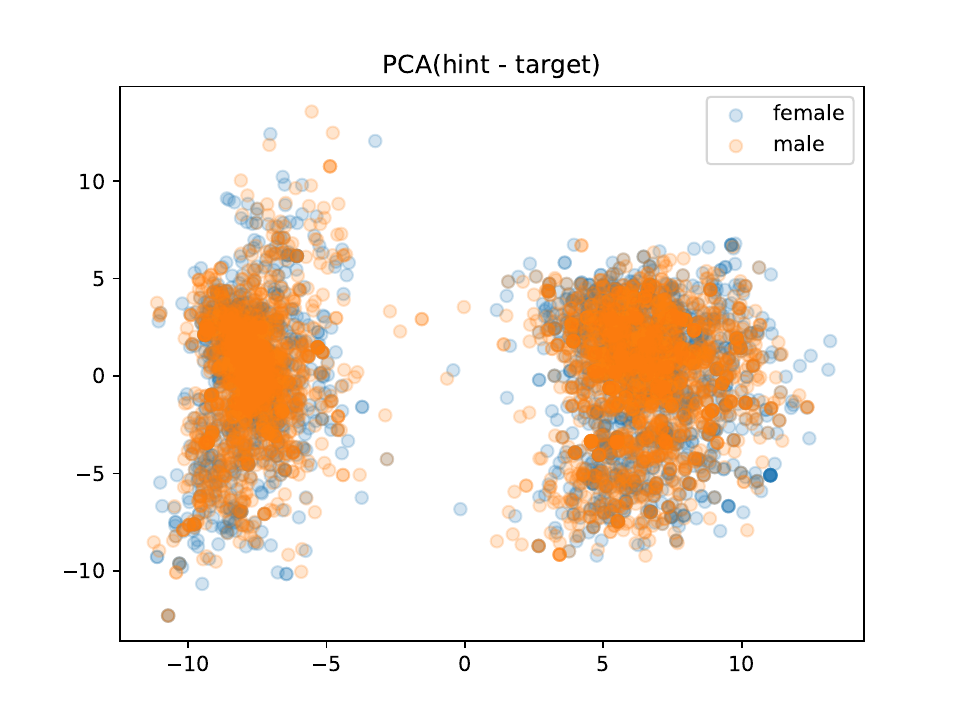}
    \caption{Gender}
    \label{fig:cos-gpt}
  \end{subfigure}
  \caption{\textbf{Scatter-plots of \textit{target-hint} difference from GPT after PCA transformation with the first 2 principal components.} Here, we attempt to align with the political leaning and gender labels.}
  \vspace{-1.5em} %
  \label{fig:pca-gender-pol}
\end{figure}
